# Supplementary material for: Quantum parallel information exchange (QPIE) hybrid network with transfer learning
Source: arXiv:2504.04235 source file (2025-04-05)
Supplement: Supplementary file 1 [file appendix.tex]

\section{Preliminary and Definition}
\subsection{Quantum Embedding}

Quantum embedding acts as encoders, facilitating the transformation of classical datasets into quantum feature maps \cite{b40}. Quantum embedding aims to overcome classical computation limits by exploiting and transferring the classical features into a quantum feature map. In quantum pre-processing, this is the vital step for quantum simulation \cite{sun2016quantum}. The quantum embedding process utilizes quantum adiabatic optimization techniques. Specifically, a quantum system initiates with an initial ansatz, evolves towards an excited energy state, and ultimately seeks optimization at the minimum Hamiltonian, corresponding to the system ground state energy (minimum loss). These quantum embedding layers transform classical information into quantum states, allowing quantum computers to process and analyze data in a manner potentially exceeding classical computational capabilities.

At the core of quantum embedding, there lies the principle of transforming classical data into a form that quantum algorithms can process. Unlike classical bits, qubits can exist in the superposition of states, allowing for the embodied comprehensive combination of all probabilities of the whole system. The basis of angle encoding maps classical data directly into the angles of quantum gates, such as rotation gates and amplitude amplification, which subsequently modulate the quantum state of qubits \cite{gianani2022experimental}. The structure includes unitary operations acting on a quantum state with the input of classical weights \cite{b41}.
\begin{equation}
    |\psi(x)\rangle = \sum_{i}^{N} \alpha_{i}(x)|i\rangle
\end{equation}
Here, \(|\psi(x)\rangle\) represents the quantum state corresponding to the classical data input $x$, \(\alpha_{i}(x)\) is the angle encoding the data, and \(|i\rangle\) are the basis states of the quantum system. For example, the multidimensional classical data is encoded into the phases of the quantum state, allowing quantum algorithms to exploit the computational advantages of quantum mechanics. The rotation of qubits acts as a tensor product with different states, 
\begin{equation}
    |\psi\rangle = \bigotimes_{i=1}^{n} R(\theta_i)|0\rangle
\end{equation}
where \(R(\theta_i)\) represents a rotation operation (e.g., \(R_x\), \(R_y\), or \(R_z\)) on the \(i\)-th qubit with \(\theta_i\) being the classical data encoded as an angle.

\subsection{Parameterized Quantum Circuit}
Similar to classic neural network \cite{b45}, the intuition of PQC provides the learning function that returns the error cost of the model for optimizing the weights so the PQC can learn the patterns of the dataset. The PQC aims to predict the labels by the given quantum-enhanced data. It represents a class of quantum circuits where certain elements, for instance, gate angles, are parameterized by tunable variables. Following quantum gates, some of which are parameterized by a set of parameters \(\vec{\theta}\). The action of a PQC on an \(n\)-qubit state 
\begin{equation}
    |\psi(\vec{\theta})\rangle = U(\vec{\theta})|0\rangle^{\otimes n},
\end{equation}
shows that the changed state equals the previous state with unitary operations acting on itself. Here \(U(\vec{\theta})\) is the unitary operation applied by the PQC, decomposable into a sequence of parameterized and non-parameterized quantum gates:
\begin{equation}
    U(\vec{\theta}) = U_m(\theta_m) U_{m-1}(\theta_{m-1}) \cdots U_1(\theta_1)
\end{equation}
Each \(U_i(\theta_i)\) represents a quantum gate parameterized by \(\theta_i\), acting on one or more qubits.

A parameterized quantum circuit is based on a series of single-gate operations. Noticed that the Variational Quantum Eigensolver (VQE) \cite{tilly2022variational} asserts the ground state energy of a Hamiltonian \(H\) is the lowest possible expectation value attainable by any quantum state. In order to minimize the expectation value on the right, hereby approximating the ground state energy \(E_0\):
\begin{equation}
    E_0 \leq \langle \psi(\vec{\theta}) | H | \psi(\vec{\theta}) \rangle,
\end{equation}
where $E_0$ denotes the ground state energy, \(|\psi(\vec{\theta})\rangle\) is the quantum state prepared by the PQC parameterized by \(\vec{\theta}\), and \(H\) is the Hamiltonian of the system. 

\subsection{Quantum Enhanced Transfer Learning}
Since current real-world datasets are mostly fixed classical bits and have a limitation of several qubits, it is significant to connect a quantum net with a feed-forward neural network. To reduce the time consumption of whole framework training by introducing transfer learning in quantum-enhanced features, a highly customized hybrid quantum model is a very convenient way to train the system. Let us consider the integration of quantum computing with transfer learning, quantum-enhanced transfer learning (QETL). For instance, a quantum state can be represented as \(|\psi\rangle = \sum_{i} \alpha_{i} |i\rangle\), where \(|i\rangle\) are basis states and \(\alpha_{i}\) are complex coefficients. Quantum operations, applied to these states, facilitate the manipulation of information in a multi-dimensional space, thereby enabling enhanced computational parallelism. Concerning our proposed model, we can map the QETL into four stages:
\begin{enumerate}
  \item \(C_{in}\) is the full-fledged pre-trained neural network that accepts classical input and maps classical input data of dimension to a quantum state in a \(\log(n)\)-dimensional Hilbert space, preparing the data for quantum processing. The classical output splits into different batches and feeds into quantum input features. 
  \item Non-sequential quantum net operates on the quantum data, utilizing quantum computational and superposition principles to process information, where the quantum embedding net contains multiple single operation gates.
  \item \(Q_{out}\) translates the quantum-processed information back to classical data.
  \item \(C_{predict}\) a linear layer of measured classical output connects a prediction layer, where the prediction layer calculates the loss based on the accuracy function.
\end{enumerate}
